# Supplementary material for: Node Connectivity Augmentation via Iterative Randomized Rounding
Source: arXiv:2108.02041 source file (2021-08-04)
Supplement: Supplementary file 1 [file appending_binary_trees.tex]

\subsection{Appending Extended Binary Trees}\label{sec:appending}

We now describe our main procedure that, given a tree $T = (V, E)$ rooted at a vertex $r$, computes a tree spanning the set $F \subseteq V$ of leaves of $T$.

We start by defining the ranking $\pi: F \to [|F|]$ of the leaves that we will use. Algorithm~\ref{alg:generate-ranking} generates a ranking that prioritizes the leaves that are closest to the root, and among them it prioritizes leaves that have more siblings that are leaves.

\begin{algorithm}
Let $Q \leftarrow \arg \min\{|P_T(r,f)|: f \in F\}$.

Let $x \in \arg\max\{|\mathtt{Sibling}_T(f) \cap F|: f \in Q\}$, breaking ties arbitrarily

$\pi(x) \leftarrow 1 + \mathtt{offset}$.

Let $p$ be the closest ancestor of $x$ such that $|\mathtt{Child}_T(p)| > 1$, if any, otherwise let $p \leftarrow \emptyset$.

\eIf{$p \neq \emptyset$}{\Return $\pi \circ \mathtt{GenerateRanking}(T[V \setminus (P_T(p,x) \setminus \{p\}  )], 1 + \mathtt{offset})$}{\Return $\pi$}

\caption{The $\mathtt{GenerateRanking}(T, \mathtt{offset})$ procedure.}
\label{alg:generate-ranking}
\end{algorithm}

The main steps of our procedure are now described in Algorithm~\ref{alg:main-alg}, whose input is a tree $T = (V, E)$ with a set of leaves $F$.

\begin{algorithm}
Pick an arbitrary root $r \in V \setminus F$. From now on, $T$ is assumed to be a tree rooted at $r$.

$\pi \leftarrow \mathtt{GenerateRanking}(T, 0)$.

$(T_0, \mathcal{B}) \leftarrow \mathtt{PartitionIntoBinaryTrees}(T)$

\For{$B \in \{T_0\} \cup \mathcal{B}$}{$G(B) \leftarrow \mathtt{GenerateLeftToRightTree}(B)$}

\Return $\mathtt{AppendTrees}\left(T_0, \mathcal{B}, \{G(B)\}_{B \in \{T_0\} \cup \mathcal{B}} \right)$

\caption{The $\mathtt{GenerateSpanningTree}(T)$ procedure.}
\label{alg:main-alg}
\end{algorithm}

Thus, all that remains to discuss in here is the $\mathtt{AppendTrees}\left(T_0, \mathcal{B}, \{G(B)\}_{B \in \{T_0\} \cup \mathcal{B}} \right)$ procedure, that takes as input a family of extended binary trees along with trees spanning their leaves, and produces a tree spanning all the leaves of the original tree $T$. In order to produce this spanning tree over $F$, we use an iterative procedure that maintains what we call a main tree, which is a subtree of $T$ that increases after each iteration, until it becomes equal to $T$. During each iteration, we consider the main tree and a tree from the family $\mathcal{B}$, and we merge their leaf-spanning trees. We call this procedure ``appending''. Reiterating, we append the trees of $\mathcal{B}$ to the main tree $T'$, which at the beginning is equal to $T_0$, one at a time, until $T' = T$.

\paragraph*{The $\mathtt{AppendTrees}(\ldots)$ procedure} 

The starting point of our analysis are Lemmas~\ref{lemma:extended-binary-tree-properties} and~\ref{lemma:extended-binary-tree-bounds}. In particular, in order to obtain the bound of Lemma~\ref{lemma:extended-binary-tree-bounds}, we assumed that all vertices other than the leafs $\{f_1, \ldots, f_m\}$ and their parents have $w$-value equal to $3$. Thus, whenever the $w$-value of such a vertex is smaller than $3$, then this vertex has some extra budget that it can use in case its $w$-value is increased by the addition of some leaf-to-leaf edge. We now make this more formal. 

Let $B = (V, E)$ be an extended binary tree rooted at a vertex $p$, whose set of leaves is $F$, and let $(f_1, \ldots, f_m)$ be the ordering generated by $\mathtt{GenerateLeftToRightOrdering}(B')$, where $B' = B[(V \setminus F) \cup \mathtt{Marked}(B)]$. For each vertex $u \in V \setminus F$, we define $\mathtt{Budget}_B(u) = \max\{H(3) - H(w(u)), 0\}$. Moreover, for $i \in \{1, m\}$, we define
\begin{equation*}
 \mathtt{Budget}_B(f_i) = 
    \begin{cases} 
      \frac{1}{3}  & \textrm{if }\mathtt{Budget}_B(\mathtt{parent}_B(f_i)) > 0, \\
      \frac{5}{12} & \textrm{if }\mathtt{Budget}_B(\mathtt{parent}_B(f_i)) = 0.
   \end{cases}
\end{equation*}

We will use the budget defined above when appending a tree $B$ to the main tree. We now do some case analysis. From now on, let $T'$ denote the main tree, let $B$ denote the tree we are about to append to the main tree, which is rooted at a vertex $p$ that is connected to a vertex $p' \in T'$ in the original tree $T$. 

We now do some case analysis.

\begin{lemma}
Let $B$ be an extended binary tree rooted at vertex $p$ that is appended to a vertex $p'$ of the main tree $T'$. Then, the new $H$-average will be at most 1.8593.
\end{lemma}
\begin{proof}

    Let $B'$ be the extended binary tree of $T'$ which $p'$ belongs to when we consider the original decomposition $\{T_0\} \cup \mathcal{B}$ of $T$ into extended binary trees. This means that $B'$ is either $T_0$ or an extended binary tree of the set $\mathcal{B}$ that was appended in a prior iteration. Before appending $B$, its leaf-spanning tree $G(B)$ has a $w$ that, by Lemma~\ref{lemma:extended-binary-tree-bounds}, has an $H$-average of at most $1.84$. Let $G(T')$ be the leaf-spanning tree of the main tree. Let $w$ denote the $w$-value of all vertices of $B$ and $T'$ before appending $B$ to $T'$, and $w'$ be the value after appending. In order to connect $G(B)$ with $G(T')$, we will add one edge between $G(B)$ and $G(T')$, based on the ``location'' of $p'$ in $B'$. In all cases, from our decomposition, we must have $|\mathtt{Child}_{B'}(p')| \geq 2$.

\begin{itemize}
    \item Case: $\mathtt{Child}_{B'}(p') = \{v_1, v_2, v_3\}$. In this case, $v_1, v_2, v_3$ must all be leaves. So the worst-case increase is incurred when $p'$ is an external node, which is $\frac{1}{4} + \frac{1}{5}$ which can easily be charged to the budget on the exterior path of $B$
    
    \item Case: $|\mathtt{Sibling}(\mathtt{marked}(p))| = 2$. In this case, there two cases for whether $p'$ is part of an external path or not. Suppose $p'$ is part of an external path with $\mathtt{Child}_{B'}(p') = \{v_1, v_2\}$, and w.l.o.g. assume that $v_1$ is on the same external path. In this case, we add the edge $(\mathtt{marked}_{B'}(v_2), \mathtt{marked}_B(p))$. The worst-case increase incurred in the path $P_{B'}(p', \mathtt{marked}_{B'}(v_2))$ is
    \begin{equation*}
        \frac{1}{3} + \frac{|P_{B'}(v_2, \mathtt{marked}_{B'}(v_2))| - 1}{4} + \frac{1}{5}.
    \end{equation*}
    if $p'$ is not part of an external path, then we add the edge $(\mathtt{marked}_{B'}(v_1), \mathtt{marked}_B(p))$ instead. The The worst-case increase incurred in the path $P_{B'}(p', \mathtt{marked}_{B'}(v_1))$ is
    \begin{equation*}
        \frac{|P_{B'}(v_2, \mathtt{marked}_{B'}(v_2))| - 1}{4} + \frac{1}{5} + \frac{1}{6}.
    \end{equation*}
    The amount of budget we have on the external path of $B$ is at least $\frac{|P_{B}(p, \mathtt{marked}_{B} (p))|}{3}$
    
    \item Case: $|\mathtt{Sibling}(\mathtt{marked}(p))| = 3$. In this case, we know by the decomposition that $|\mathtt{Sibling}(\mathtt{marked}(B'_{v_1}))| = |\mathtt{Sibling}(\mathtt{marked}(B'_{v_2}))| = 3$ where $\mathtt{Child}_{B'}(p') = \{v_1, v_2\}$. If $p'$ and $v_1$ are part of the external path of $B'$, then we add the edge $(\mathtt{marked}_{B'}(v_2), \mathtt{marked}_B(p))$, if $p'$ is not part of the external path then we add the edge $(\mathtt{marked}_{B'}(v_1), \mathtt{marked}_B(p))$. The worst case increase incurred in $B'$ is either $\frac{1}{3}$ or $\frac{1}{4}$ depending on if $p'$ is part of the external path of $B'$ or not plus
    \begin{equation*}
        \frac{|P_{B'}(v_2, \mathtt{marked}_{B'}(v_2))| - 2}{4} + \frac{1}{5} + \frac{1}{6}
    \end{equation*}

    \item $p'$ is part of an external path of $B'$. We do some further case analysis:
        \begin{itemize}
            \item $\mathtt{Child}_{B'}(p') = \{v_1, v_2\}$ and moreover, $B'_{v_1} \prec B$ and $B'_{v_2} \prec B$. Wlog, assume that $v_1$ is part of the external path of $B'$. In this case, we add the edge $(\mathtt{marked}_{B'}(v_2), \mathtt{marked}_B(p))$. The worst-case increase incurred in the path $P_{B'}(p', \mathtt{marked}_{B'}(v_2))$ is
            \begin{equation*}
                \frac{1}{3} + \frac{|P_{B'}(v_2, \mathtt{marked}_{B'}(v_2))| - 1}{4} + \frac{1}{5}
            \end{equation*}
            Regarding the path $P_{B}(p,\mathtt{marked}_B(p))$, we use the budget of the vertices of the path, and do some case analysis for the last two vertices, $f_1 \coloneqq \mathtt{marked}_B(p))$ and its parent. In the case where $w(\mathtt{parent}_B(f_1))=  2$, the increase on all vertices of the path $P_B(p,\mathtt{parent}_B(f_1))$ can be paid by the budget of each vertex, and so is the increase for the vertex $f_1$, which is either $1/3$ or $1/4$. We will now use the budget of the path 
        \end{itemize}

    \item then if we charge the entire increase to JUST the exterior nodes of $B$ including the 3-stars at its leaves we get the following formula for the new cost of these nodes
        \[
            \frac{1}{2q+3}\left( (q+2)H(2)+(q-2)H(3)+2H(4)+\frac{1}{3} +\frac{q-2}{4}+\frac{1}{5} +\frac{1}{6} \right)
        \]
    \item this formula is maximized for $q=3$ with $1.8592592$
\end{itemize}
\end{proof}

\begin{lemma}
    Let $B$ be an extended binary tree rooted at vertex $p$, with $q=2$, and is appended to a vertex $p'$ of the main tree $T'$. Then, the new $H$-average $T'$ will be at most $1.87921807$.
\end{lemma}
\begin{proof}
    Again, the $H$-average of  $B$ before it is appended to $T'$ is at most $1.84$. 
    
    If $|P_{T'}(p',\mathtt{marked}_{T'}(p'))| = 2$, that is, the level of the node $\mathtt{marked}_{T'}(p')$ is one higher than $\mathtt{marked}_{T'}(p)$ when we attach $B$. Then the worst case is when $p'$ has two children and $B$ has only $3$ nodes. The total cost to the nodes of $B$ in this case is $((H(3)+H(4)+2H(2) + \frac{1}{3}+\frac{1}{4})/4 = 1.875$
    
    Now we consider $|P_{T'}(p',\mathtt{marked}_{T'}(p'))| + 1 = 3$, again the worst case is when $B$ has 3 leaves. Therefore, both the exterior leaves of $T'_{p'}$ have two siblings. 

    the idea here is to charge the increase due to appending $B$ to the nodes on the path it connects to. the worst case here is again when the depth of the parent subtrees are both 3, and thus must have 3-stars at the bottom. therefore, the worst case increase is $1/3 + 1/4 + 1/5 + 1/6$. this cost averaged across the nodes of $B$ will be 
    \[
        \frac{1}{4}\left( 2H(2)+H(3)+H(4)+\frac{1}{3} +\frac{1}{5}+\frac{1}{6} \right) = 1.901417
    \]
    So this is a bad approach, consider instead also charging to the parent of $B$. Since the depth from the parent of $B$ is $3$, the previous lemma applies, so the parent has at most $1.8592592$ charged to it. This means that averaging this way gives
    \[
        \frac{1}{5}\left( 2H(2)+H(3)+H(4)+\frac{1}{3} +\frac{1}{5}+\frac{1}{6} +1.8592592 \right) = 1.895185173...
    \]
    again, not great. so consider charging to the whole path from $p$ to the node we connect to, including the siblings. 
    \[
    \frac{1}{9}\left( 2H(2)+H(3)+H(4)+\frac{1}{3} +\frac{1}{5}+\frac{1}{6} + 5*1.8592592 \right) = 1.87921807
    \]
\end{proof}

The next case does not affect the previous since it requires that the parent has at least 2 leaves in order to be feasible. 
\begin{lemma}
    Let $B$ be an extended binary tree rooted that is just the vertex $\{p\}$, and is appended to a vertex $p'$ of the main tree $T'$. Then, the new $H$-average $T'$ will be at most $1.89337445925$
\end{lemma}
\begin{proof}
    Since $B$ is a single node, we know by our decomposition that $p'$ must already have at least $3$ children. If $u$ is the marked child of $p'$, then we know that the worst-case $w$-values of $p'$ and $u$ are $3$ and $4$ respectively if $p'$ is an external node. By applying the previous lemma and distributing the increase in cost to $B$, $p'$ and $p$, we have that the cost of $T'$ increases to at most 
    \[
    \frac{1}{5}\left( H(2)+\frac{1}{4} +\frac{1}{5} + 4*1.87921807 \right) = 1.89337445925
    \]

\end{proof}

\begin{lemma}
    Let $B$ be an extended binary tree rooted at vertex $p$ that is appended to a vertex $p'$ of the main tree $T'$. Then, the new $H$-average will be at most $1.84365079$ if we allow limited rewiring of the leaf-to-leaf tree of $T'$.
\end{lemma}
\begin{proof}
    This rewiring is done when $B$ is to be appended and the leaf-to-leaf edge $(v,\mathtt{marked}_B(p))$ will be added. So only nodes with depth from root at least as low as $p'$ will have been rewired. So this rewiring is the first time any nodes on $T'_{p'}$ will have been rewired.

    The limited rewiring will occur when we add edge $(\mathtt{marked}_{T'}(p'),\mathtt{marked}_B(p))$ to the leaf-to-leaf tree. Let $u$ be the grandparent of $\mathtt{marked}_{T'}(p')$, and assume $u$ is an interior node. Suppose $u$ has two children $u_1$ and $u_2$ and $\mathtt{marked}_{T'}(p')\in T'_{u_1}$. By the left-to-right tree construction and since no rewiring has been done below $p'$ we know that $T_{v_2}$ will exactly have two leaf-to-leaf edges incident to it, $\{u,\mathtt{marked}_{T'}(v_2)\}$ and $\{x, \mathtt{marked}_{T'} (v_2)\}$ for some $x\in T'$. The rewiring is to delete the edge $\{x, \mathtt{marked}_{T'} (v_2)\}$ and add edge $\{x, v\}$. This rewiring will change the cost of the tree its in by at least $\frac{1}{5}+\frac{1}{6} - \frac{1}{4}-\frac{1}{5} = -\frac{1}{12}$. When we then append $B$ after this the increase changes in these last to nodes from $\frac{1}{5}+\frac{1}{6}$ to instead being $\frac{1}{6}+\frac{1}{7}-\frac{1}{12}$ which is enough to get the desired bound. 
    
    If $u$ does not have $2$ children, then $u$ has a budget of $1/3$ and this can be used instead when $B$ is appended. If a tree is appended at $p'$ again after $B$ is appended, the leaf-to-leaf edge added will be incident to $\mathtt{marked}_{T'}(p')$ and the same path that $B$ increased, this is a low cost, at most $1.8314814$

\end{proof}

\begin{lemma}
    Let $B$ be an extended binary tree rooted at vertex $p$, with $|P_{p,\mathtt{marked}_B(p)}| = 2$, that is appended to vertex $p'\in T'$. Then the new $H$-average of $T'$ will be at most $1.869047619$
\end{lemma}
\begin{proof}
    We are interested in the cases here that lead to $B$ having a cost greater than or equal to the stated bound. There are only so many cases cases
    
    \begin{enumerate}
   
        \item If $p'$ has two children that are leaves. $p$ has 3 children that are leaves. 1.875
        \item if $p'$ has two children that are leaves. $p$ has 2 children. not as bad as previous case
        \item if $p'$ has three children that are leaves. obviously not as bad as previous cases.
        \item $p'$ has 4 grandchildren. $B$ is two leavse
        \item $p'$ has more than 4 granchildren. $B$ is two leaves. 1.844444...
        \item $p'$ has more than 4 granchildren. $B$ is 3 leaves. even better
        \item $p'$ has 6 grandkids and $b$ is 3 leaves. charge to whole path you connect to. 
        \item $p'$ has 6 grandkids and has been used before. $B$ is 3 leaves. 1.869047619
     \end{enumerate}
\end{proof}

\begin{lemma}
    Let $B$ be an extended binary tree rooted at vertex $p$, with $|P_{p,\mathtt{marked}_B(p)}| = 1$, that is appended to vertex $p'\in T'$. Then the new $H$-average of $T'$ will be at most $1.885238$  
\end{lemma}  
\begin{proof}
    
\end{proof}

\begin{lemma}\label{lemma:decreasing-depth}
    The order of the trees we append is monotonically increasing with respect to distance from the root. 
\end{lemma}

\begin{algorithm}
    Let $T' = T_0$;\\
    Let $G' \coloneqq \mathtt{GenerateLeftToRightTree}(T')$;
    
    \For{each $B \in \mathcal{B}_1$}
    {
        $G(B) \coloneqq \mathtt{GenerateLeftToRightTree}(B)$;\\
        Set $\mathtt{marked}_1(root(B)) \coloneqq \ell_1(B)$.\\
        Set $\mathtt{marked}_2(root(B)) \coloneqq \ell_m(B)$.
    }
    
    \While{$(\mathcal{B}_1 \neq \emptyset)$}
    {
        Pick $(B,p') \in \mathcal{B}_1$ such that $p' \in T'$, and $p'$ is maximal amongst all such $p'\in T'$\\
        $\mathcal{B}_1 \coloneqq \mathcal{B}_1 \setminus \{(B,p')\}$.
        
        \If{$p' \in T_0$ and $w(p') =2$}
        {
            $G' \coloneqq G' \cup G(B) \cup \{(\ell_1(B), \mathtt{marked}_1(p'))\}$
        }
        
        \eIf{If $w(p')\geq 3$ but $p'$ has been used to append another tree before or $w(p')=2$ and $deg_{T'}(p') \geq 3$}
        {
            $G' \coloneqq G' \cup G(B) \cup \{(\ell_1(B), \mathtt{marked}_2(p'))\}$\\
            If $marked_2(p')$ has not been rewired, then rewire.
        }
        {
            $G' \coloneqq G' \cup G(B) \cup \{(\ell_1(B), \mathtt{marked}_1(p'))\}$\\
            If $marked_1(p')$ has not been rewired, then rewire.
        }
    }
    \Return{(T',G')}
\caption{Appending binary trees with $SP$-value at least $2$, one at a time}
\end{algorithm}
\label{alg:main-algorithm}

\paragraph{The Second Phase of the Algorithm.} Once we have run the first phase of the algorithm and appended every tree $B\in\mathcal{B}$ with $SP(B)\geq 2$, it remains to add the trees in $\mathcal{B}$ that possess a single Steiner node. In the first phase of the algorithm, we append the trees one by one and charge the increase in cost to the appended tree $B$. In this second phase we will instead append the remaining trees in groups and charge the increase to the whole group simultaneously. 
\begin{algorithm}
    \begin{enumerate}
        \item Input: $(T', G')$ from phase 1 of the algorithm
        \item While $(\mathcal{B} \neq \emptyset)$
        \begin{enumerate}
            \item Pick $(B_1,p'), (B_2,p'), \dots, (B_n,p')\in \mathcal{B}$, all trees in $\mathcal{B}$ that share a particular parent $p'$
            \item Set $\mathcal{B}\coloneqq \mathcal{B} \setminus \{(B_1,p'),(B_2,p'),\dots, (B_n,p')\}$
            \item Generate terminal-spanning trees $G_1,\dots,G_n$ for $B_1,\dots,B_n$ respectively
            \item Set $G' \coloneqq G'\cup \left(\cup_{i=1}^n G_n \right) \cup \left (\cup_{i=1}^n \{ \mathtt{marked}(p'),\mathtt{marked}(p_i)\}\right)$, where $p_i$ is the Steiner node of $B_i$
            \item Set $T' \coloneqq T' \cup \left(\cup_{i=1}^n B_n \right) \cup \left(\cup_{i=1}^n \{(p',p_i)\}\right)$
        \end{enumerate}
        \item Return $(T', G')$
    \end{enumerate}
\end{algorithm}
